# Supplementary material for: XR-MBT: Multi-modal Full Body Tracking for XR through Self-Supervision with Learned Depth Point Cloud Registration
Source: arXiv:2411.18377 source file (2024-11-27)
Supplement: Supplementary file 1 [file extended_visual_pc_results_source.tex]

\begin{figure}
\centering
\sbox0{\includegraphics{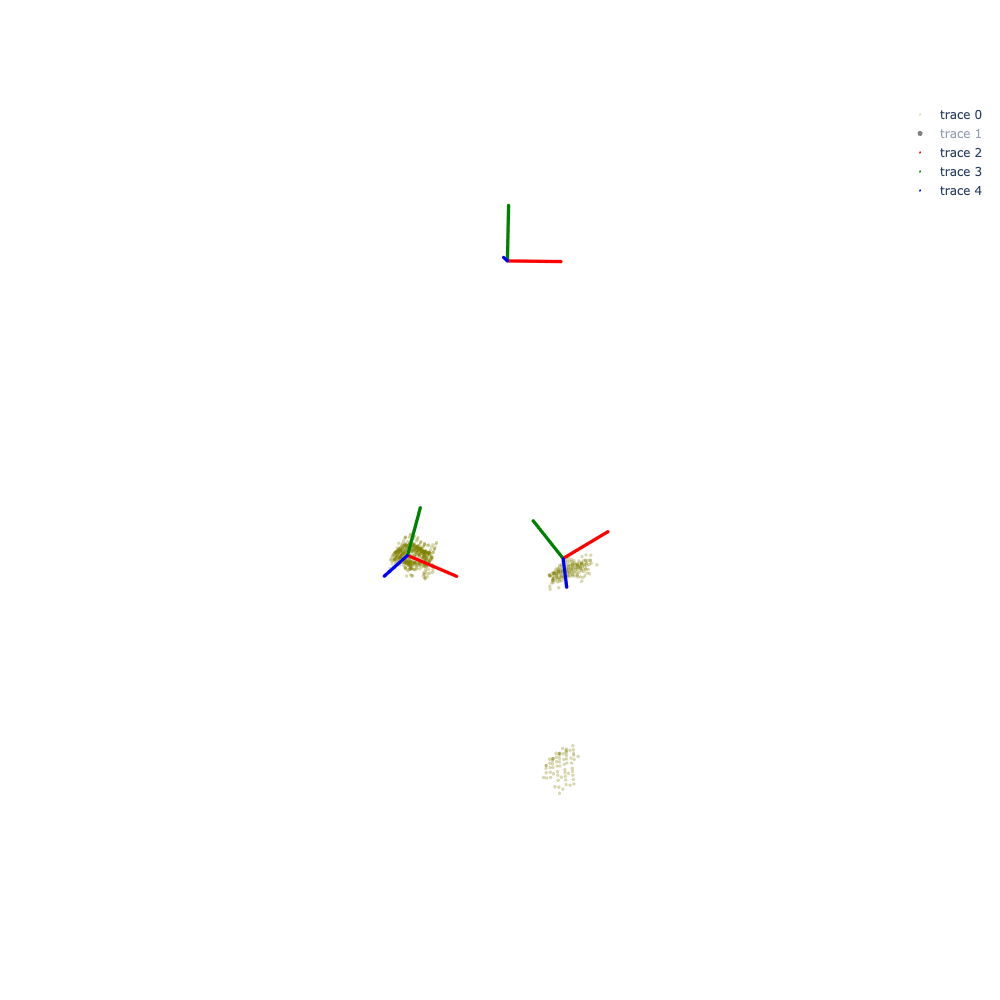}}%
\begin{subfigure}{.28\textwidth}
    \centering
    \includegraphics[height=4.5cm]{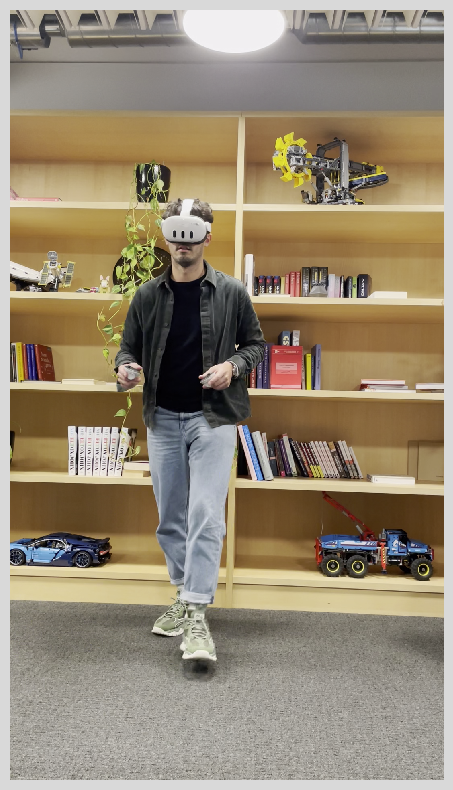}  
\end{subfigure}
\begin{subfigure}{.28\textwidth}
    \centering
    \includegraphics[clip,trim={.2\wd0} 0 {.2\wd0} 0,height=4.5cm]{supmat/figures/images/ex1_raw.png}  
\end{subfigure}
\begin{subfigure}{.28\textwidth}
    \centering
    \includegraphics[clip,trim={.2\wd0} 0 {.2\wd0} 0,height=4.5cm]{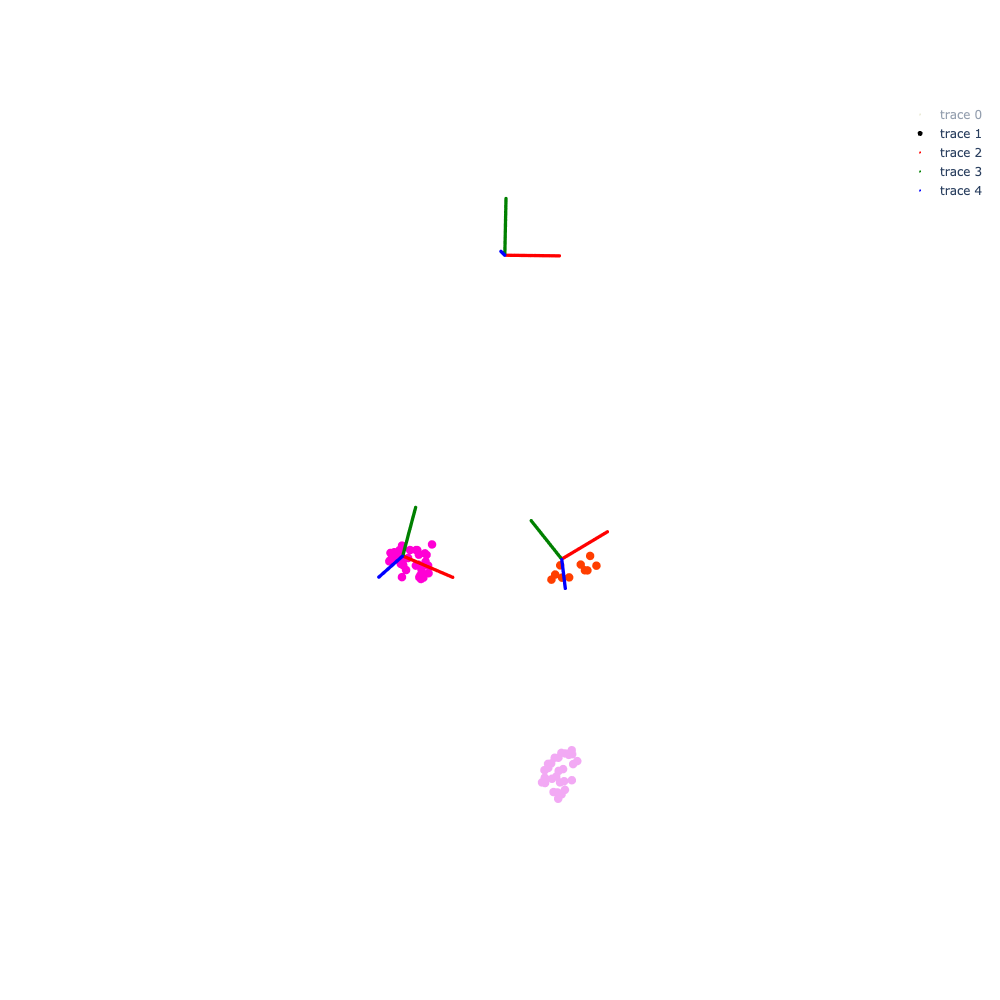}  
\end{subfigure}
\par
\begin{subfigure}{.28\textwidth}
    \centering
    \includegraphics[height=4.5cm]{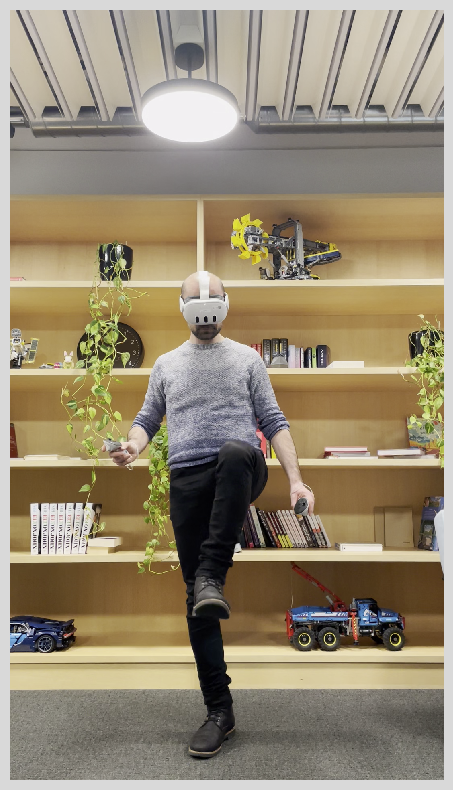}  
\end{subfigure}
\begin{subfigure}{.28\textwidth}
    \centering
    \includegraphics[clip,trim={.2\wd0} 0 {.2\wd0} 0,height=4.5cm]{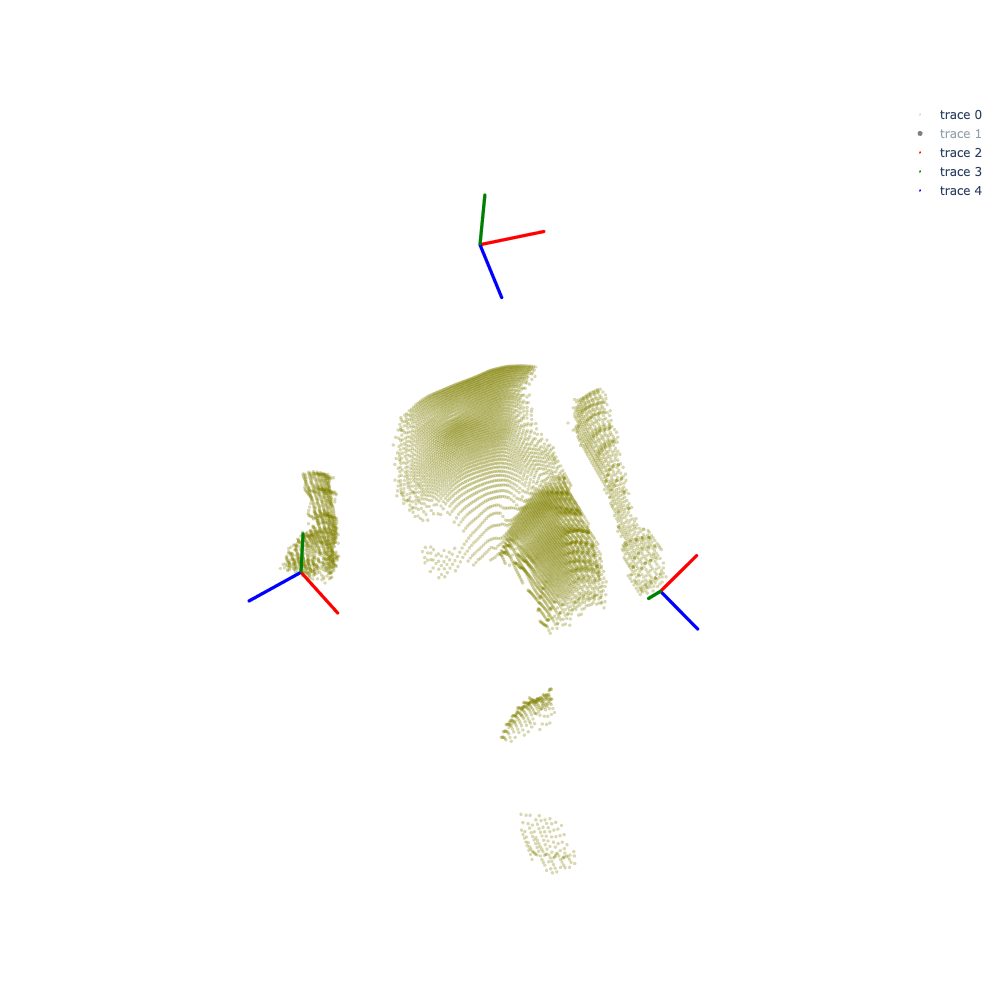}  
\end{subfigure}
\begin{subfigure}{.28\textwidth}
    \centering
    \includegraphics[clip,trim={.2\wd0} 0 {.2\wd0} 0,height=4.5cm]{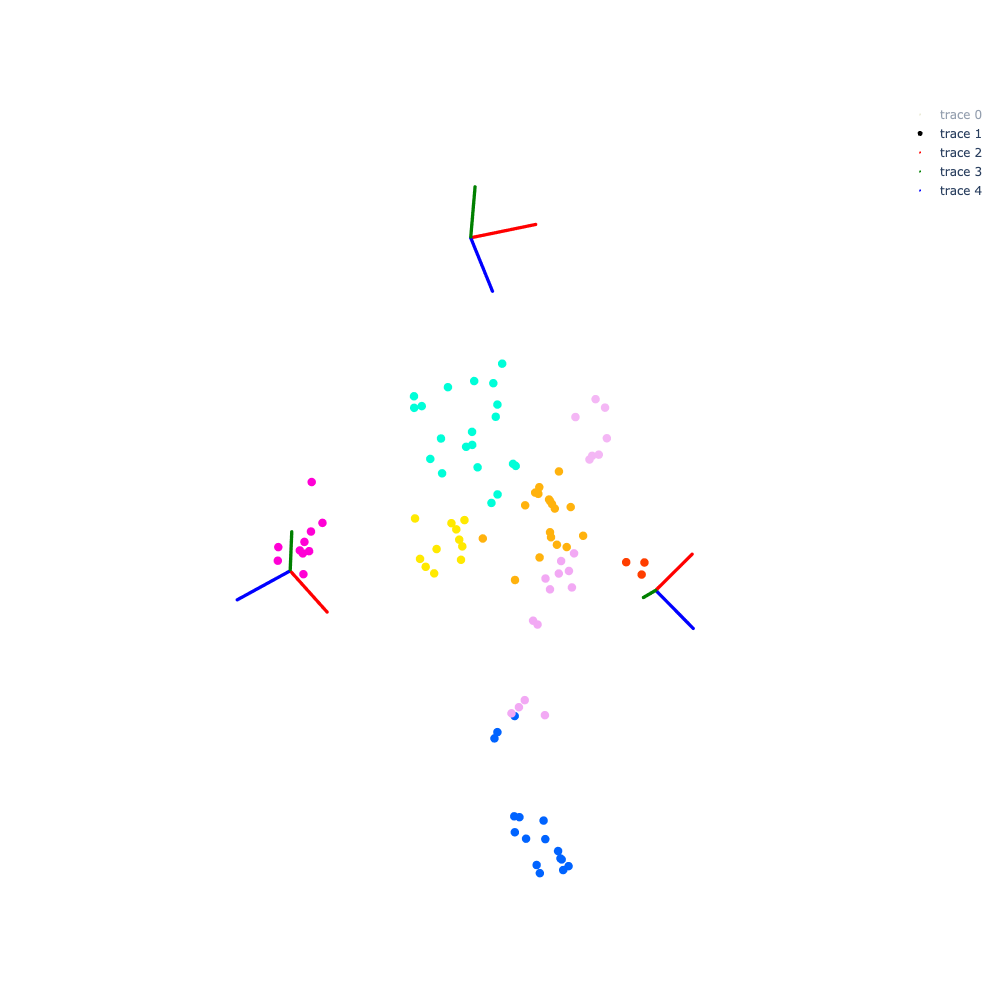}  
\end{subfigure}
\caption{Additional point cloud labelling results.}
\label{fig:extended_visual_pc_results}
\end{figure}
